# Supplementary material for: Discovering Latent Covariance Structures for Multiple Time Series
Source: arXiv:1703.09528 source file (2019-05-22)
Supplement: Supplementary file 1 [file 7-appendix-old.tex]

\onecolumn
\makeatother
\vbox{
% \hsize \textwidth
% \linewidth\hsize
% \vskip 0.1in
% %top title bar
% \hrule height 4pt
% \vskip 0.25in
% \vskip -\parskip%
\centering
{\LARGE\bf Supplementary Material for\\Discovering Explainable Latent Covariance Structures for Multiple Time Series \par}
% \vskip 0.29in
% \vskip -\parskip
% \hrule height 1pt
% \vskip 0.09in%

%authors
% \begin{tabular}[t]{c}\bf\rule{0pt}{24pt}
%         Anonymous Author(s) \\
%         Affiliation \\
%         Address \\
%         \texttt{email} \\
%       \end{tabular}%
     
}
\appendix

\section{Related Work}
\input{4-related-work.tex} 

\section{Base kernels and search grammar in the ABCD framework}
\label{appendix:base}
The below table contains base kernels described in~\cite{Lloyd2014ABCD}.
\begin{center}
\begin{tabular}{l | l | c}
Base Kernels & Encoding Function  & $k(x,x')$\\
\hline
White Noise (\textsc{WN}) & Uncorrelated noise & $\sigma^2 \delta_(x,x')$ \\
Constant (\textsc{C}) & Constant functions & $\sigma^2$ \\
Linear (\textsc{LIN}) & Linear functions & $\sigma^2 (x - l)(x - l')$\\
Squared Exponential (\textsc{SE}) & Smooth functions & $\sigma^2 \exp (-\frac{(x - x')^2}{2l^2})$\\
Periodic (\textsc{PER}) & Periodic functions & $\sigma^2 \frac{\exp(\frac{\cos \frac{2\pi(x-x')}{p}}{l^2}) - I_0(\frac{1}{l^2})}{\exp(\frac{1}{l^2}) - I_0(\frac{1}{l^2})}$ \\
\end{tabular}
\end{center}
Changepoint (CP) operator between two kernel functions:
\begin{equation*}
\begin{split}
\textrm{CP}(k_1, k_2) &= k_1 \times \boldsymbol{\sigma} + k_2 \times \overline{\boldsymbol{\sigma}}.
\end{split}
\end{equation*}
where $\boldsymbol{\sigma}(x,x') = \sigma(x)\sigma(x')$ with $\sigma(x) = \nicefrac{1}{2}(1+\tanh(\nicefrac{l-x}{s}))$ and $\overline{\boldsymbol{\sigma}}(x,x') = (1-\sigma(x))(1 - \sigma(x'))$.\\
Changewindows (CW) operator between two kernel functions:
$$\textrm{CW}(k_1, k_2) = k_1 \times \boldsymbol{\sigma}_1 \times \overline{\boldsymbol{\sigma}}_2 + k_2 \times \overline{\boldsymbol{\sigma}}_1 \times \boldsymbol{\sigma}_2.$$
where a similar definition as in $\boldsymbol{\sigma}$ can be done for $\boldsymbol{\sigma}_1, \boldsymbol{\sigma}_2$.

The language of models (or kernels) is presented by a set of rules in the grammar:
\begin{align*}
\mathcal{S} &\rightarrow \mathcal{S + B} &&\mathcal{S} \rightarrow \mathcal{S \times B} \\
\mathcal{S} &\rightarrow \mathrm{CP}(\mathcal{S,S}) &&\mathcal{S} \rightarrow \mathrm{CW}(\mathcal{S,S})  \\
\mathcal{S} &\rightarrow \mathcal{B}  
\end{align*}
where $\mathcal{S}$ represents any kernel subexpression, $\mathcal{B}$ and $\mathcal{B}'$ are base kernels~\cite{Lloyd2014ABCD}.



\section{\Acrlong*{vi} of \acrshort*{lgp}}
\label{appendix:vi_lgp}
In this section, we will give the exact form of~\acrshort*{elbo} in~\acrshort*{lgp} as well as the parameter updates in the maximizing step of variational inference. Let us recall the form of~\acrshort*{elbo} as
$$ \mathcal{L} = \expect_\vZ[\log p(\vZ)] + \expect_\vF[\log p(\vF)] + \expect_{\vZ,\vF}[\log p(\vX|\vZ,\vF)] + H[q].$$
The first term $\expect_\vZ[\log p(\vZ)]$ can be obtained as in~\cite{vibp_Doshi} for either finite case (involving the Beta prior) and infinite case (constructing via stick-breaking manner). The second quantity $\expect_\vF[\log p(\vF)]$ are the summation of the followings
$$\mathbb{E}_\vF [\log p(\vf_{k})] =  -\frac{1}{2}(\log |2\pi \vC_k| + \tr{(\vC_k^{-1}\vS_k)} + \vm_k^\top \vC_k^{-1}\vm_k),$$
with index $k$ running from $1$ to $K$. Next, $\expect_{\vZ,\vF}[\log p(\vX|\vZ,\vF)]$ is factorized into $N$ terms in the form of
\begin{equation*}
\begin{split}
\expect_{\vZ,\vF}&[\log p(\vx_{n}| \vz_{n}, \vF)] = -\frac{D}{2} \\&  -\frac{1}{2\sigma_n^2} \left(\vx_{n}^\top\vx_n -2 \sum_{k = 1}^K\nu_{nk} \vm_k^\top \vx_{n} + 2 \sum_{k < k'}\nu_{nk}\nu_{nk'} \vm_k^\top \vm_{k'} + \sum_{k = 1}^K \nu_{nk}(\tr(\vS_k) + \vm^\top_k \vm_k) \right).
\end{split}
\end{equation*}
The evaluation of $H[q]$ consists of computing $H[q(\vZ)]$(see~\cite{vibp_Doshi}) and $H[q(\vF)]$ (use the entropy of multivariate Gaussian distribution). 

For the parameter updates related to $\vZ$, readers may refer to~\cite{vibp_Doshi}. For the case of $\vm_k$, the typical coordinate ascent in variational inference corresponds to maximize the following function~\cite{DBLP:WainwrightJ08}
\begin{equation}
\label{opti_problem}
\begin{split}
\log q(\vf_{k}) &= \expect_{\vZ,\vF_{-k}}[\log p(\vX, \vZ,\vF)] + c = \expect_{\vF_{-k}}[\log p(\vF)] + \expect_{\vZ,\vF_{-k}}[\log p(\vX|\vZ,\vF)] + c\\
&=  -\frac{1}{2}\vf_{k}^\top \left( \vC_k^{-1} + \sum_{n=1}^N\frac{\nu_{nk}}{\sigma^2_n}\vI \right)\vf_{k} 
%\\ &
+ \vf_{k}^\top \left(\sum_{n=1}^N \frac{\nu_{nk}}{\sigma^2_X}  \left(\vx_{n} - \sum_{l:l\neq\ k} \nu_{nl}\vm_l \right) \right) + c,
\end{split}
\end{equation}
where $c$ is constant, $\vF_{-k}$ is the feature matrix without $\vf_k$. From (\ref{opti_problem}), the closed form solution is obtained by finding the critical point of the derivative of the above quantity. It turns out that we update $\vm_k$ = 
$\vS_k\left(\sum_{n=1}^N\frac{\nu_{nk}}{\sigma^2_X}  \left(\vx_{n} - \sum_{l:l\neq\ k} \nu_{nl}\vm_l \right) \right),$ where
$\vS_k$ is updated first as $\left(\vC_k^{-1} + \sum_{n=1}^N\frac{\nu_{nk}}{\sigma^2_n}\vI \right)^{-1}$.

\section{\Acrlong*{vi} of \acrshort*{lkm}}
\label{appendix:vi_lkm}

\paragraph{Optimal weights for the expectation over $\vZ$ of the data-fit term} 
To make it easy to follow, we restart with the bound %which is the result from the expected value of inverse matrices
\begin{align*}
\vx_n^\top \left( \sum_{k=1}^K w_{nk} \frac{1}{w_{nk}} \left(z_{nk}\vC_k + \frac{\sigma_n^2}{K}\vI\right) \right)^{-1}\vx_n 
\leq \vx^\top_n \sum_{k=1}^K w_{nk}^2 \left(z_{nk}\vC_k + \frac{\sigma^2_n}{K}\vI  \right)^{-1} \vx_n.
\end{align*} 

Here, we distribute uniformly $\sigma^2_n\vI$ to each $z_{nk}\vC_k$ to make sure that $(z_{nk}\vC_k + \frac{\sigma_n^2}{K}\vI)$ is a non-zero matrix whichever value of $z_{nk}$ is chosen (0 or 1). Taking the expectation over $\vZ$ and arrange terms, we have
\begin{align*}
\expect_\vZ \left[ \vx_n^\top \left( \sum_{k=1}^K w_{nk} \frac{1}{w_{nk}} \left(z_{nk}\vC_k + \frac{\sigma_n^2}{K}\vI\right) \right)^{-1}\vx_n  \right] &
\leq \vx^\top_n \sum_{k=1}^K w_{nk}^2 \expect_{z_{nk}} \left[ \left(z_{nk}\vC_k + \frac{\sigma^2_n}{K}\vI  \right)^{-1}\right] \vx_n.
\end{align*} 
Each term $\expect_{z_{nk}} \left[ \left(z_{nk}\vC_k + \frac{\sigma^2_n}{K}\vI  \right)^{-1}\right]$ can be evaluated straightforwardly as $\nu_{nk}\left(\vC_k + \frac{\sigma^2_n}{K}\vI  \right)^{-1} + (1 - \nu_{nk})\frac{K}{\sigma_n^2}\vI$. Let $a_{nk} =\expect_\vZ \left[ \left(z_{nk}\vC_k + \frac{\sigma^2_n}{K}\vI  \right)^{-1}\right]$.  We set up a constraint optimization problem as follows, for each $n$,
$$\min_{w_{nk}} \sum_{k=1}^{K} a_{nk} w_{nk}^2   \qquad \text{such that} \qquad \sum_{k=1}^{K} w_{nk} =1, \quad w_{nk} > 0, \quad k = 1\dots K. $$

We then obtain the Lagrange multiplier for this problem
$$L(\mathbf{w}, \lambda) = \sum_{k=1}^{K} a_{nk} w_{nk}^2  - \lambda \sum_{k=1}^{K} w_{nk}$$
The derivative solution of $\partial L / \partial w_{nk}$ is $w_{nk}=\lambda / 2a_{nk}$. Considering that the sum of all $w_{nk}$ should be $1$, we obtain 
$$\lambda = \frac{1}{\frac{1}{2} \sum_{k=1}^K a_{nk}^{-1} }.$$ 
Finally, we get the optimal solution as
$$w_{nk} = \frac{a_{nk}^{-1}}{\sum_k a_{nk}^{-1}}.$$

\paragraph{Evidence Lower Bound}
The optimal weights retrieved from the previous section is used to construct the~\acrshort{elbo} of~\acrshort{lkm} as follow.
\begin{align*}
	\log p(\vX) \geq &  \expect_{\vZ}[\log p(\vZ)] + H[q] 
	\underbrace{
	  -\frac{1}{2} \left( \sum_{n=1}^N \sum_{k = 1}^K w_{nk}^2 a_{nk} + \log \left|2\pi \left(\sum_{k=1}^K \nu_{nk}\vC_k + \sigma_n^2 \vI \right) \right| \right)}_{\expect_{\vZ}[\log p(\vX|\vZ)]}
\end{align*}

We can obtain $\expect_{\vZ}[\log p(\vZ)]$ and $H[q]$ ($q$ in this case is just $q(\vZ)$) in a similar way with~\acrshort*{lgp}. 

\paragraph{Parameter updates via optimization}The closed-form update for $\nu_{nk}$ in \acrshort*{lgp} does not hold, replacing by a gradient-based optimization on the obtained \acrshort*{elbo}. Here, we parameterize $\nu_{nk}$ by a sigmoid function $\nu_{nk} = 1 / (1 + \exp(-\xi_{nk}))$ which corresponds the canonical parameterization of the Bernoulli distribution, keeping $\nu_{nk} \in (0,1)$. The GP hyperparameter optimization is performed along side the variational parameters.

The implementation of~\acrshort*{lkm} develops on GPflow~\cite{GPflow2017} library which operates on Tensorflow computation~\cite{tf}. We make the source code available at \url{<anonymized>}.

\section{Likelihood $p(\vX|\vZ)$ of \acrshort*{lgp}}
This section gives the details obtaining the likelihood $p(\vX|\vZ)$. This is a necessary step to prove the well-definedness of ~\acrshort*{lgp}.


The distribution $p(\vX|\vZ,\vF)$ of $\vX$ given $\vZ, \vF$ and $\sigma_X$ (WLOG we can assign all $\sigma_n$  equal to $\sigma_X$) is
\begin{equation}
\label{eq:X_give_Z_F}
\begin{split}
% &\frac{1}{(2\pi \sigma_X^2)^{ND/2}} \exp \{
p(\vX|\vZ,\vF) = (2\pi \sigma_X^2)^{-ND/2} \exp \{-\frac{1}{2\sigma_X^2}\tr((\vX{-}\vZ\vF)^\top(\vX{-}\vZ\vF))\},
\end{split}
\end{equation}
where $\tr(\cdot)$ is the trace of matrix. Since each row $\vf_{k}$ in $\vF$ representing a feature is placed a GP prior with covariance kernel $\vC_k$
$$p(\vf_{k}) = (2\pi)^{-D/2}|\vC_k|^{-1/2}\exp(-\frac{1}{2}\vf_{k}^\top \vC_k^{-1}\vf_{k}),$$
where $|\cdot|$ denotes the determinant of matrix. Since these features are independent, the prior distribution $p(\vF)$ over $\vF$ is constituted from the product of $p(\vf_{k}|\vC_k)$
\begin{equation}
\label{eq:F_prior}
 p(\vF) = (2\pi)^{-KD/2} \prod_{k =1}^K |\vC_k|^{-1/2}
\exp(-\frac{1}{2}\sum_{k=1}^K \vf_{k}^\top \vC_k^{-1} \vf_{k}).
\end{equation}

As we mentioned in the main text, $p(\vF)$ is not truly Gaussian but the distributions of its individual rows $p(\vf_k)$ are. To fit with the Gaussianity of $p(\vX|\vZ,\vF)$, we use the vectorization on matrix $\vF$. The exponentiated term in (\ref{eq:F_prior}) can be written as
$
\sum_{k=1}^K \vf_{k}^\top \vC_k^{-1} \vf_{k} {=} {\vectorize(\vF^\top)^\top}{\bigoplus_{k=1}^K \vC^{-1}_k \vectorize(\vF^\top)},
$
where $\vectorize(\cdot)$ is the vectorization which transforms a matrix into a column vector by stacking the columns of a matrix, $\bigoplus$ is the direct sum operation of matrix. This quantity can be understood as a Gaussian distribution $p(\vectorize(\vF))$ and illustrated in Figure~\ref{fig:matrix f}.
 \begin{figure}
 \input{./figures/illustrate_prior_F.tex}
 \caption{Illustration of representing $\sum_{k = 1}^K\vf_{k}^\top\vC^{-1}_k \vf_{k}$. The first row vector is the concatenation of $\vf_{k}^\top$, being written as $\vectorize(F^\top)^\top$. The block matrix is a block diagonal matrix where the block at diagonal position are $\vC_k^{-1}$. The last column vector is the transpose of the first row vector.
 }
 \label{fig:matrix f}
 \end{figure}

%We carefully investigate the exponential expression when multiplying equations (\ref{eq:X_give_Z_F}) and (\ref{eq:F_prior}). Our aim is to marginalize out $\vF$ to get the likelihood $p(\vX|\vZ) = \int p(\vX|\vZ,\vF)p(\vF)d\vF$. The exponentiated term in $p(\vX|\vZ)$ should be manipulated to have a quadratic form of $\vF$ to make the integration tractable. 
%%% REMOVE TO GET MORE SPACE
% One direction is to convert the equation (\ref{eq:exp_f}) to the form of trace of matrix $\tr(\sum_{k=1}^K Fc_k^{-1}F^T\Delta_k)$. However, there exists a dimensional disagreement between two matrices in trace where this matrix is a $K \times K$ matrix while the one in (\ref{eq:X_give_Z_F}) is a matrix $D\times D$. Even performing the cyclic permutation in trace, we still cannot get a good form to proceed the derivation. The more effective solution is to transform trace forms in (\ref{eq:X_give_Z_F}) into vectorization. %%%%%%%%%%%%%%%%%%%%
Next, we rewrite $p(\vX|\vZ,\vF)$ using the new representation of $\vF$ as $\vectorize(\vF)$. Some algebraic properties~\footnote{\tiny Cyclic permutation: $\tr(\vA\vB\vC) = \tr(\vB\vC\vA) = \tr(\vC\vA\vB)$;\\
 	Trace to vectorization: $\tr(\vA^\top \vB) = \vectorize(\vA)^\top\vectorize(\vB)$;\\ 
 	Vectorization to Kronecker product:  $\vectorize(\vA\vB\vC) = (\vC^\top \otimes \vA)\vectorize(\vB)$}
between trace and vectorization are applied to get the followings:
\begin{equation*}
\begin{split}
{\tr (\vX^\top \vZ \vF)} &{=} \tr(\vF \vX^\top \vZ) {=}  \vectorize (\vF^\top)^\top \vectorize(\vX^\top \vZ); \\
{\tr (\vF^\top \vZ^\top  \vX)} &{=}\tr(\vZ^\top \vX \vF^\top){=}  \vectorize (\vX^\top \vZ)^\top \vectorize(\vF^\top),
\end{split}
\end{equation*}
where the invariance of cyclic permutation of trace and the conversion from trace to vectorization are used respectively;
\begin{equation*}
\begin{split}
{ \tr [(\vZ \vF)^\top (\vZ\vF)]} =&\tr[(\vZ\vF)(\vZ\vF)^\top] \\
=& \vectorize(\vF^\top \vZ^\top)^\top \vectorize(\vF^\top \vZ^\top)\\
% = & [(Z \otimes I_D) \vectorize(F^T)]^T[(Z \otimes I_D ) \vectorize(F^T)] \\
= &\vectorize(\vF^\top)^\top (\vZ^\top \vZ \otimes \vI) \vectorize(\vF^\top),
\end{split}
\end{equation*}
% \begin{equation*}
% \begin{split}
% { \tr [(ZF)^T (ZF)]} =&\tr[(ZF)(ZF)^T] =\vectorize(F^TZ^T)^T \vectorize(F^TZ^T)
% % = & [(Z \otimes I_D) \vectorize(F^T)]^T[(Z \otimes I_D ) \vectorize(F^T)] \\
% = \vectorize(F^T)^T (Z^TZ \otimes I_D) \vectorize(F^T),
% \end{split}
% \end{equation*}
where the first two '='s are done as the same as the previous derivation, then the vectorization is written in the form of Kronecker product. Note that $\otimes$ is the Kronecker product. By using the above results and the technique of completing the square, we get the exponentiated term in $p(\vX|\vZ,\vF)p(\vF)$
\begin{equation}
\label{eq:exp}
\begin{split}
p(\vX|\vZ,\vF)p(\vF) = & \tr \{\frac{1}{\sigma^2_X}(\vX - \vZ\vF)^\top (\vX-\vZ\vF) \}  + \sum_{k=1}^K \vf_{k}^\top \vC^{-1}_k \vf_{k} \\
 =  & \underbrace{\frac{1}{\sigma^2_X}\tr(\vX^\top \vX) - \frac{1}{\sigma^2_X}\vectorize(\vX^\top\vZ)^\top \vG\vectorize(\vX^\top \vZ)}_{(a)} 
  \\
 	&
    + \underbrace{(\vG\vectorize(\vX^\top \vZ)  - \vectorize(\vF^\top))^\top \frac{\vG^{-1}}{\sigma_X^2}(\vG\vectorize(\vX^\top \vZ) - \vectorize(\vF^\top))}_{(b)},
\end{split}
\end{equation}
% \begin{equation}
% \label{eq:exp}
% \begin{split}
% &\underbrace{\frac{1}{\sigma^2_X}\tr(X^TX) - \frac{1}{\sigma^2_X}\vectorize(X^TZ)^TG\vectorize(X^TZ)}_{(a)} \\
% & + \underbrace{(G\vectorize(X^TZ)  - \vectorize(F^T))^T \frac{G^{-1}}{\sigma_X^2}(G\vectorize(X^TZ) - \vectorize(F^T))}_{(b)},
% \end{split}
% \end{equation}
where $\vG = ( \vZ^\top \vZ \otimes \vI  + \sigma_X^2\bigoplus_{k=1}^K \vC^{-1}_k)^{-1}$. 
% To have a better understanding about the structure of matrix $G$, we illustrate $G^{-1}$ in Figure \ref{fig:block matrix} \anh{removed figure to save space}.
% %%%%%%%%%%%%%%%%
% \begin{figure}
% \centering
% % \resizebox{0.5\textwidth}{!}{%
% \input{./figures/illustrate_G.tex}
% \caption{Block matrix visualization of $G^{-1}$. Here $u_{ij}$ is the element at $i$-th row and $j$-th column of the matrix $Z^TZ$}
% \label{fig:block matrix}
% \end{figure}%%%%%%%%%%%%%%%%
Equations (\ref{eq:X_give_Z_F}), (\ref{eq:F_prior}) and (\ref{eq:exp}) lead to the likelihood function by integrating out $\vF$ since (b) in (\ref{eq:exp}) makes the integration tractable; only (a) left in the likelihood function $p(\vX|\vZ)$

\begin{equation*}
\begin{split}
p(\vX|\vZ) = & \int p(\vX|\vZ,\vF)P(\vF) d\vF \\
 = &\frac{1}{(2\pi)^{(ND+KD)/2} \sigma_X^{ND}\prod_{k=1}^K \sqrt[]{|\vC_k|}} \exp \left\{-\frac{1}{2\sigma^2_X}\tr(\vX^\top \vX) + \frac{1}{2\sigma^2_X}\vectorize(\vX^\top \vZ)^\top \vG\vectorize(\vX^\top \vZ)\right\} \\
& \int \exp \left\{-\frac{1}{2}(\vG\vectorize(\vX^\top \vZ)  - \vectorize(\vF^\top))^\top (\sigma_X^2\vG)^{-1} (\vG\vectorize(\vX^\top \vZ) - \vectorize(\vF^\top)) \right\}d\vF \\
=& \frac{\sqrt[]{2\pi^{KD}|\sigma^2_X \vG|}}{(2\pi)^{ND/2} \sigma_X^{ND}\prod_{k=1}^K \sqrt[]{|\vC_k|}} \exp \left\{-\frac{1}{2\sigma^2_X}\tr(\vX^\top \vX) + \frac{1}{2\sigma^2_X}\vectorize(\vX^\top \vZ)^\top \vG\vectorize(\vX^\top \vZ)\right\} \\
=& \frac{1}{(2\pi)^{ND/2} \sigma_X^{ND - KD}\sqrt[]{|(\vI \otimes \vZ^\top \vZ +\sigma_X^2\sum_{k=1}^K \vC^{-1}_k\otimes \Delta_k)| \prod_{k=1}^K |\vC_k |}} \\
&\exp \left\{-\frac{1}{2\sigma^2_X}\tr(\vX^\top \vX) + \frac{1}{2\sigma^2_X}\vectorize(\vX^\top \vZ)^\top \vG\vectorize(\vX^\top \vZ)\right\}.
\end{split}
\end{equation*}
We rewrite the likelihood as follows:
\begin{equation}
\label{eq:likelihood}
\begin{split}
p(\vX|\vZ)= & \frac{(2\pi)^{-ND/2} \sigma_X^{KD - ND}}{\sqrt[]{|(\vZ^\top \vZ \otimes \vI  +\sigma_X^2\bigoplus_{k=1}^K \vC^{-1}_k)| \prod_{k=1}^K |\vC_k |}}\\
&\exp \{\frac{1}{2\sigma^2_X}[-\tr(\vX^\top \vX) + \vectorize(\vX^\top \vZ)^\top \vG\vectorize(\vX^\top \vZ) 
] \}.
\end{split}
\end{equation}
\textbf{Remark on the connection to the MAP asymptotic approach} Note that when observing the likelihood function is that the MAP asymptotic of~(\ref{eq:likelihood}) falls back to the same form of feature allocation $\tr(\vX^\top(\vI - \vZ(\vZ^\top \vZ)^{-1}\vZ^\top)\vX)$ presented in~\cite{BroderickKJ13}. From~(\ref{eq:likelihood}), we have
\begin{align*}
&p(\vX, \vZ) = p(\vX|\vZ)p(\vZ)\\
&= \frac{(2\pi)^{-ND/2} \sigma_X^{KD - ND}}{\sqrt[]{|(\vZ^\top \vZ \otimes \vI  +\sigma_X^2\bigoplus_{k=1}^K \vC^{-1}_k)| \prod_{k=1}^K |\vC_k |}}
\exp \{\frac{1}{2\sigma^2_X}[-\tr(\vX^\top \vX) + \vectorize(\vX^\top \vZ)^\top \vG\vectorize(\vX^\top 
\vZ) 
] \} \\
&\times \frac{\gamma^{K_+} \exp\{\sum_{n=1}^N \frac{\gamma}{n}\}}{\prod_{h=1}^H \tilde{K}_h!} \prod_{k=1}^{K_+}\frac{(S_{N,k} -1)! (N - S_{N,k})!}{N!}.
\end{align*}
When we set $\gamma := \exp(\lambda /(2\sigma_X^2))$  and take limit $\sigma_X^2 \rightarrow 0$ for the logarithm of $p(\vX,\vZ)$, we have
\begin{align*}
-2\sigma_X^2 \log p(\vX,\vZ) \sim \tr(\vX^\top \vX) - \vectorize(\vX^\top \vZ)^\top (\vZ^\top \vZ\otimes \vI) \vectorize(\vX^\top \vZ) + K_{+} \lambda^2.
\end{align*}
Here we can write $\vectorize(\vX^\top \vZ)^\top (\vZ^\top \vZ\otimes \vI)^{-1} \vectorize(\vX^\top \vZ) = \tr(\vX^\top \vZ(\vZ^\top \vZ)^{-1}
\vX)$. Now we get the same objective as the collapsed BP-means in~\cite{BroderickKJ13}.  Although our derived likelihood $p(\vX|\vZ)$ shows a strong connection to the standard feature allocation via the asymptotic view, this asymptotic analysis has not had a clear algorithmic contribution to learn~\acrshort*{lgp} yet.


\section{Well-definedness of \acrshort*{lgp} and \acrshort*{lkm}}
\label{appendix:well_define}
\begin{prop}
	The likelihood of \acrshort*{lgp} $p(\vX|\vZ)$ in Eq.~\ref{eq:likelihood} is well-defined.
\end{prop}
\begin{proof}
We are going to show that if the number of columns goes to infinity, the distribution in (\ref{eq:likelihood}) is still well-defined. To validate this, we perform \textit{lof} on $\vZ$. All nonzero features are accumulated on the left, denoted as $\vZ_+$; the rest of columns are zero vectors, denoted as $\vZ_0$. $\vZ_+$ has $K_+$ columns, $\vZ_0$ has $K_0$ columns and $K = K_+ + K_0$. Note that $K_+$ is finite. The determinant in (\ref{eq:likelihood}) is written as
\begin{equation}
\begin{split}
|  \vZ^\top \vZ \otimes  \vI + \sigma_X^2\bigoplus_{k=1}^K \vC^{-1}_k|
= &|\begin{bmatrix}
\vZ^\top_+ \vZ_+ & 0 \\
0 & 0
\end{bmatrix}
\otimes \vI
+ 
\sigma^2_X \bigoplus_{k \in K_+} \vC^{-1}_k \oplus \bigoplus_{k \in K_0} \vC^{-1}_k
| \\
 = &\sigma^{2K_0D}_X\prod_{k \in K_0} |\vc_k^{-1}|  |  \vZ^\top_+ \vZ_+ \otimes \vI + \sigma^2_X\bigoplus_{k \in K_+} \vC^{-1}_k|.
\end{split}
\end{equation}
The term $\prod_{k \in K_0} |\vC_k^{-1}|$ will be canceled out since the existence of $\prod_{k =1}^K |\vC_k|$ in the denominator of (\ref{eq:likelihood}). The same can be done for $\sigma^{2K_0D}_X$ by taking a root square first then eliminating by $\sigma^{KD}_X$. The remaining terms $\prod_{k \in K_+} |\vC_k|$ and $\sigma^{K_+D}_X$ are finite.
Also, the term containing $\vZ$ in the exponentiated expression of (\ref{eq:likelihood}) is written as
\begin{equation}
\vectorize(\vX^\top \vZ)^\top \vG\vectorize(\vX^\top \vZ) =\vectorize(\vX^\top \vZ_+)^\top (\vZ^\top_+ \vZ_+ \otimes \vI + \sigma^2_X\bigoplus_{k \in K_+} \vC^{-1}_k)^{-1}\vectorize(\vX^\top \vZ_+)
\end{equation}
is finite.
\end{proof}

\begin{prop}
	The likelihood of~\acrshort*{lkm} is well-defined.
\end{prop}
\begin{proof}
	In the case of~\acrshort*{lkm}, the likelihood can be easily obtained since there is no participation of latent feature variables
	$$p(\vX|\vZ) = \prod_{n=1}^N p(\vx_n | \vz_{n}).$$
	
	Analogously, the \emph{lof} operator is applied on $\vZ$ to get $\vZ_{+}$. Each row in $\vZ_{+}$ is used to generate kernel $\vD_n = \sum_{z_{nk} \in \vZ_{+}}z_{nk}\vC_k + \sigma_n^2\vI$ which is now the finite sum of covariances kernels $\vC_k$. Thus, each multivariate Gaussian likelihood $p(\vx_n | \vz_{n})$ has a well-defined covariance. Finally, we can conclude that $p(\vX|\vZ)$ is well-defined.
\end{proof}

\section{Synthetic data}
\begin{table}[H]
      \centering
%       \scalebox{0.60}{
\begin{tabular}{l|l}
 Generating kernel & Found kernel \\ \hline
$\textrm{LIN} {+} \textrm{SE}$ 
				&      $\textrm{SE}  {+} \textrm{LIN} {+} \textrm{SE} {\times} \textrm{LIN}$       \\ \hline
$\textrm{LIN}{+} \textrm{LIN} {\times} \textrm{SE}$          				    &    SE + SE         \\ \hline
$\textrm{LIN}{+} \textrm{LIN} {\times} {\textrm{SE}} {+} \textrm{PER}$ 
	&      {SE} + {LIN} + {SE} + {LIN${\times}$LIN} + {SE${\times}$PER}   \\ 
\end{tabular}
% }
\caption{Comparing the true generated kernel with the found structure}
\label{tab:syn}
\end{table}
 We generate synthetic three time-series according to several chosen kernels to verify our kernel selection algorithm. Each time series consists of 200 data points, generated from different kernels (see Table \ref{tab:syn}). 

Although the generated data seems similar in terms of global shapes, the data has clear differences in terms of local structures. The first column of  Figure~\ref{fig:simple} show the three generated time series. It is easy to notice that all time series share  trending shapes with smoothing caused by LIN and SE kernels. However, the first time series has more LIN trending component than the second. In addition, PER kernel is one of the components playing the role of creating the periodicity in the third time series. 

The decomposition from this synthetic data can be visually seen in Figure~\ref{fig:simple}, and discovered kernels are in Table~\ref{tab:syn}. Although the synthetic data shared the LIN structure, it looks like having smoothness more than having a clear LIN trending. The discovered kernel from the first time series contains the LIN structure but is dominant by the smoothness of global structures among three times series. One of the interesting observations is that the \acrshort*{lgp} can distinguish the PER kernel of the third time series in form of the product with SE. 

\section{\Gls*{fe}}
\label{sec:fe}

Every structure in the additive kernel set is expanded together. The generated structures will be unified into a single set (see Fig.~\ref{fig:expansion} for comparison FE and PE). The model comparison is done between search depths.

\begin{figure}
	\centering
    \scalebox{0.9}{
		\input{./figures/expansion.tex}
    }
	\caption{Structure search strategies. (a) Partial expansion (PE). (b) Full expansion (FE).}
	\label{fig:expansion}
\end{figure}


We report the additional result of our models running on~\acrshort*{fe} mode in Table~\ref{tab:fe}.\\

\begin{table}
      \centering
	\begin{tabular}{@{}c|ccc|ccc|c@{}}
			& 3 stocks & 6 stocks & 9 stocks & 2 houses & 4 houses & 6 houses & 4 currencies \\ \midrule \midrule
			Spike and Slab & 1.80     & 2.81     & 10.26     & 13.95    & 8.59    & 11.33    & 151.37       \\
			GPRN & 0.49     & 3.76     & 6.30     & 12.96    & 11.07    & 8.84    & \underbar{117.05}       \\
			\acrshort*{abcd}           & 0.40      & 3.69     & 8.35     & 6.58     & 5.84     & 7.96     & 330.00       \\
			\acrshort*{rabcd}          & \underbar{0.38}     & \textbf{1.22}     & \underbar{4.85}     & \underbar{2.75}     & \underbar{2.22}     & \underbar{3.10}     & 210.56       \\
			\midrule
			%\textit{SM}             & \textbf{0.35}     & 1.43     & \textbf{4.14}     & 5.72     & 3.13     & 4.26     & 158.17       \\
			\acrshort*{lgp}    & \textbf{0.36}        & \underbar{1.47}        & \underbar{4.82}      & \textbf{2.15}        & \textbf{2.08}        & \textbf{2.28}        & \textbf{81.98} \\
			\acrshort*{lkm}    & \underbar{0.38}        & 1.69        & \textbf{4.30}      & \underbar{2.62}       &  2.54  
			& 3.42
			& \textbf{57.74} \\            
		%\textit{SM}             & \textbf{0.35}     & 1.43     & \textbf{4.14}     & 5.72     & 3.13     & 4.26     & 158.17       \\ 
        \midrule  
		\acrshort*{fe}-\acrshort*{lgp}  & \textbf{0.35}    & 1.84     & 6.35     & 5.07     & 4.87     & 7.30     & \textbf{59.40}        \\
		\acrshort*{fe}-\acrshort*{lkm}  & \textbf{0.36}    & 1.70     &\textbf{ 4.24}     & 4.46     & 3.97     & 6.73     & \underbar{100.59} 	\end{tabular}
	\caption{RMSEs on all data sets with corresponding methods. FE-gpLFM and FE-LKM are the experiment settings running in FE mode.}
	\label{tab:fe}
\end{table}



\section{Comparison report}
\label{apendix:comparison}
\paragraph{Subprime Mortgage in US house data}The subprime mortgage happened around 2007 and dropped until 2009. The bold texts in the following report roughly describe this event.
\begin{figure}[H]
\centering
\includegraphics[width=0.9\textwidth]{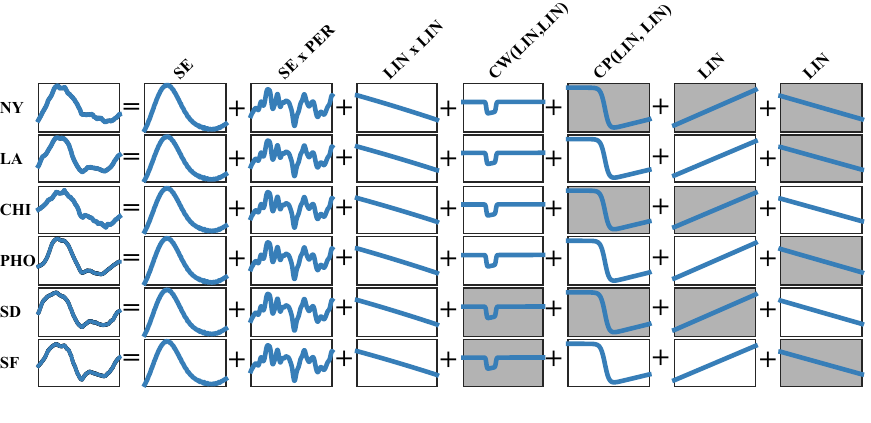}
\caption{The decomposition of housing prices in six cities: New York (NY), Los Angeles (LA), Chicago (CHI), Phoenix (PHO), San Diego (SD), San Francisco (SF).}
\end{figure}

\noindent\fbox{%
    \parbox{0.98\textwidth}{%
    \textbullet\ NY and LA and  CHI and PHO and SD and SF share the following properties \\
$\triangleright$ This component is a smooth function with a typical lengthscale of 1.8 years\\ 
\textbullet\ NY and LA and  CHI and PHO and SD and SF share the following properties \\
$\triangleright$ This component is very approximately periodic with a period of 153.0 years.Across periods the shape of this function varies smoothly with a typical lengthscale of 3.4 months.Since this lengthscale is small relative to the period this component may more closely resemble a non-periodic smooth function\\ 
\textbullet\ NY and LA and  CHI and PHO and SD and SF share the following properties \\
$\triangleright$ This component is a quadratic polynomial\\ 
\textbullet\ NY and LA and  CHI and PHO share the following properties \\
$\triangleright$ This component is linearly decreasing.This component applies until \textbf{Oct. 2006} and from \textbf{Jan. 2008} onwards\\ 
\textbullet\ LA and PHO and SF share the following properties \\
$\triangleright$ This component is linearly increasing.This component applies until Jun 2008\\ 
\textbullet\ LA and PHO and SF share the following properties \\
$\triangleright$ This component is linearly increasing\\
\textbullet\  CHI and SD share the following properties \\
$\triangleright$ This component is linearly decreasing
    }}    

\paragraph{Currency exchange of emerging markets}
We bring up the report for four currencies (South African Rand, Indonesian Rupiah, Malaysian Ringgit, Russian Rouble) as an example\\
\begin{figure}[H]
	\centering
	\includegraphics[width=0.9\textwidth]{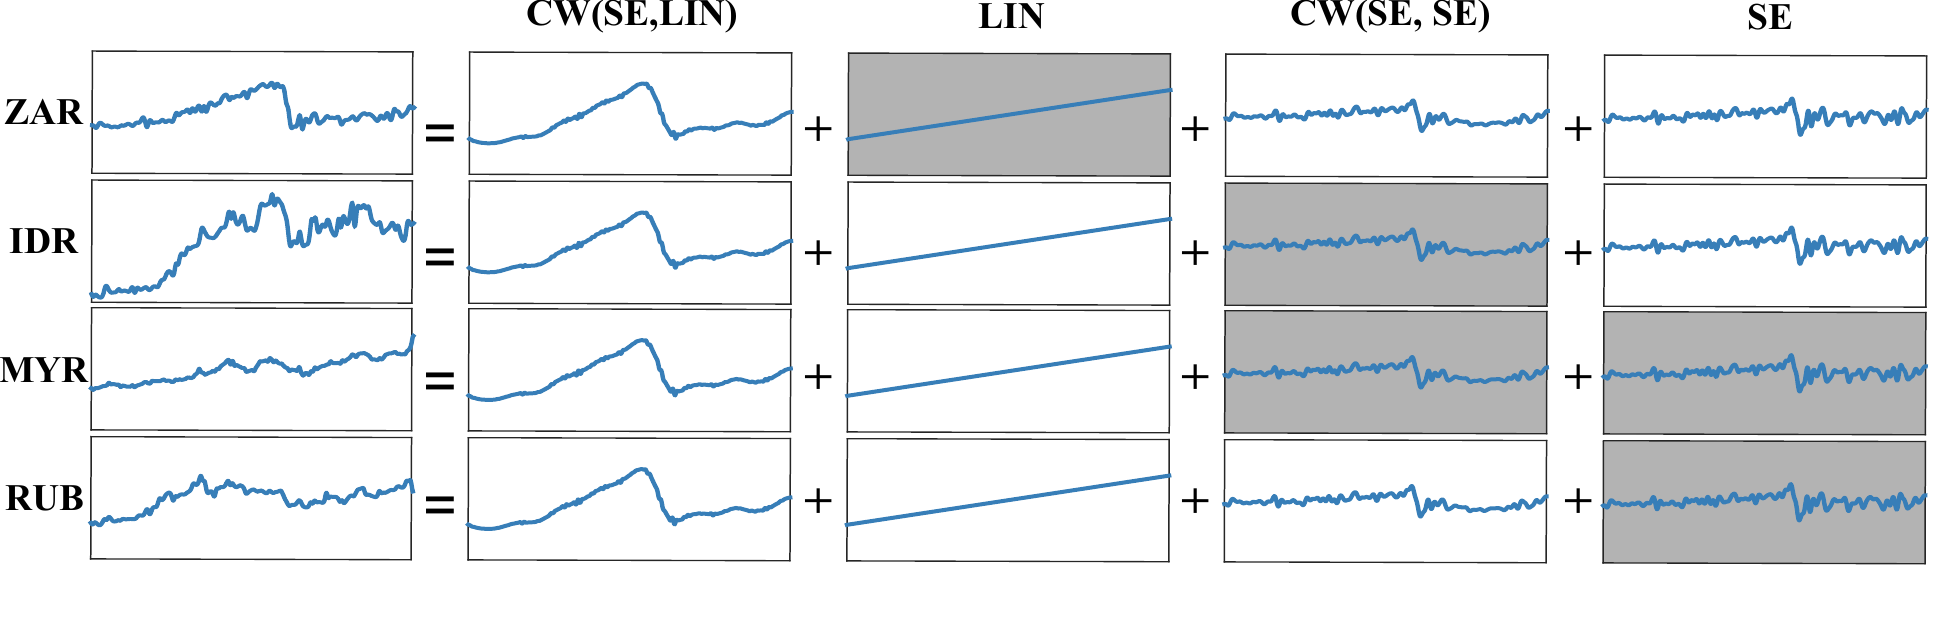}
	\caption{The decomposition of four currencies: South African Rand (ZAR), Indonesian Rupiah (IDR), Malaysian Ringgit (MYR), Russian Rouble (RUB). The shaded ones are inactive components.}
	\label{fig:currency}
\end{figure}

 \noindent\fbox{%
 	\parbox{0.98\textwidth}
 	{%
 		\textbullet\  South African Rand and Indonesian Rupiah and  Malaysian Ringgit and Russian Rouble share the following properties\\
 		$\triangleright$ This component is a smooth function with a typical lengthscale of 6.4 days.This component applies until \textbf{Sep. 15th 2015} and from \textbf{Sep. 17th 2015} onwards.\\
 		\textbullet\    Indonesian Rupiah and  Malaysian Ringgit and Russian Rouble share the following properties\\
 		$\triangleright$ This component is linearly increasing. 
 		\\
 		\textbullet\   South African Rand and Russian Rouble share the following properties\\
 		$\triangleright$ This component is a smooth function with a typical lengthscale of 29.6 hours.This component applies until \textbf{Oct. 22nd 2015} and from \textbf{Nov. 10th 2015} onwards. \\
 		\textbullet\    South African Rand and Indonesian Rupiah share the following properties\\
 		$\triangleright$ This component is a smooth function with a typical lengthscale of 28.1 hours.
 	}%
 }
